# Supplementary material for: Geometry-Driven Detection, Tracking and Visual Analysis of Viscous and Gravitational Fingers
Source: arXiv:1911.12383 source file (2020-08-19)
Supplement: Supplementary file 1 [file a_appendix.tex]

We note the density field by $f$: $\mathbb{R}^3 \to \mathbb{R}$. In Fig.~\ref{fig:derivative-approximation}, the blue points represent midpoints of voxels. The density values at blue points are observed and given by the data. In this work, we approximate derivatives of $f$ at midpoints by two alternative methods as follows. Without the loss of generality, we illustrate how to estimate the derivatives at the red-circled point of Fig.~\ref{fig:derivative-approximation} noted as $\vect{p_0}=(x_{1,0}, x_{2,0}, x_{3,0})$. 

\remark{
\textbf{Method One\quad} We take the estimation of the partial derivative with respect to $x_1$ coordinate at the red-circled point as an example. The adjacent two orange points in Fig.~\ref{fig:derivative-approximation}a are $h$ units away from the red-circled midpoint $\vect{p_0}$ along the $x_1$ coordinate; the density values of the two orange points are $f(x_{1,0}+h,x_{2,0},x_{3,0})$ and $f(x_{1,0}-h,x_{2,0},x_{3,0})$ respectively. Then, we use the central difference formula to estimate the derivative at $\vect{p_0}$: 
\begin{dmath} \label{equa:first_order_derivative_x}
\frac{\partial f}{\partial x_1}(\vect{p_0}) \approx f_{x_1}(\vect{p_0},h) =
f_{x_1}(x_{1,0},x_{2,0},x_{3,0},h) = \frac{f(x_{1,0}+h,x_{2,0},x_{3,0})-f(x_{1,0}-h,x_{2,0},x_{3,0})}{2h}
\end{dmath}
Let $s$ be the the side length of voxel. When $h$ equals $s$, the orange points overlap with two adjacent blue points of the red-circled point. Hence, we use densities at the two adjacent blue points directly to estimate the partial derivative with respect to $x_1$; namely, we let $h$ equate $s$ for Equation~\ref{equa:first_order_derivative_x} to acquire the partial derivative. Partial derivatives for other coordinates are estimated similarly by using their corresponding central differences and letting $h$ equate $s$. The result is shown in the leftmost column of Fig~\ref{fig:results-fingering}. 
}

\textbf{Method Two\quad} We also test the facet model \cite{haralick1983ridges} which approximates coefficients of the Taylor polynomial locally by using least squares method. We use the Taylor polynomial $g$, Equation~\ref{equa:taylor-polynomial}, to approximate the density function $f$ near the red-circled point $\vect{p_0}$ of Fig.~\ref{fig:derivative-approximation}b locally. The unknown parameters are the terms of $\nabla f(\vect{p_0})$ and the elements of $H(\vect{p_0})$. In Fig.~\ref{fig:derivative-approximation}b, given the densities of the blue points near the red-circled point, to acquire the unknown parameters, we use the least squares method to optimize the following function: 
\begin{equation}
minimize \sum_{\vect{p} \in \mathscr{P}}{(g(\vect{p})-f(\vect{p}))^2}
\end{equation}
where $\mathscr{P}$ is a set of midpoints that are close to the red-circled point $\vect{p_0}$. The results of this method for the finger core extraction are displayed in the rightmost column of Fig.~\ref{fig:results-fingering}. 

\remark{
\textbf{Results on synthetic data\quad} We test both the methods mentioned above on synthetic data. The volume rendering of the synthetic data is shown in Fig.~\ref{fig:synthetic-volume}. The columnar and spiral shapes have higher densities in their central regions. The results for the two methods on this data are shown in the leftmost and rightmost of Fig.~\ref{fig:results-synthetic} respectively. Method One, when $h$ equals $s$, produces curvilinear features that are similar to the facet model (Method Two); these curvilinear features are confirmed to be ridge voxels. 
}

\remark{
\textbf{Summary\quad} From this study, it is observed that Method One, when $h$ equals $s$, and Method Two are both able to extract ridge voxels from the synthetic data (Fig.~\ref{fig:results-synthetic}). However, for the fingering data, the finger cores produced by Method One in Fig~\ref{fig:results-fingering} are more continuous than the finger cores detected by Method Two, the facet model. Hence, in our system, we use Method One as the default technique for the extraction of finger cores. 
}

% When $h=10^{-5}$ voxel size, each of the detected feature is almost each individual spiral column. Thus, we can separate spiral columns in the synthetic data and extract each individual spiral column based on the results when  $h=10^{-5}$  voxel size by using the same watershed-based segmentation method when we separate fingers. 
