# Supplementary material for: Geometry-Driven Detection, Tracking and Visual Analysis of Viscous and Gravitational Fingers
Source: arXiv:1911.12383 source file (2020-08-19)
Supplement: Supplementary file 2 [file b_appendix.tex]

\remark{
Method One of the derivative approximation fixes $h$ to be $s$, the side length of voxel, and acquires ridge voxels. However, if we use the ridge voxels directly to be the finger cores in this application, specific branching structures of fingers may be missing, which is shown in the leftmost of Fig~\ref{fig:results-fingering} and demonstrated in Sect.~\ref{sect:finger_core_extraction}. 
% According to the study of Damon \cite{damon1999properties}, ridges do not represent branching structures well theoretically, and the branching structures may be close spatially but disconnected when represented by ridges. 
To remedy this, in this appendix, we adjust the spacing parameter $h$ for the extraction of finger cores, and explain the adjustment of $h$ produces equivalent results as the adjustment of $r$ in Sect.~\ref{sect:finger_core_extraction}. 
% To remedy this for this application, we acquire more connections of finger branches by incorporating more voxels that are near ridges in finger cores; to implement this idea, we adjust the spacing parameter $h$ for the extraction of finger cores as follows. 
When $h$ is smaller than $s$, we estimate the densities of the orange points in Fig.~\ref{fig:derivative-approximation}a through the tri-linear interpolation of densities of nearby blue points. The results with varying values of $h$ for finger core extraction are shown on the left side of Fig~\ref{fig:results-fingering}. Intuitively, when $h$ is equal to $s$, the extracted thin features are ridge voxels; when $h$ becomes smaller than $s$, the resulting features become thick by expanding from ridge voxels to preserve more branching connections. The same phenomenon is observed for the synthetic data in Fig.~\ref{fig:results-synthetic} as well. 
% The adjustment of $h$ is flexible for the finger extraction because domain scientists can control the values of $h$ to acquire finger cores by trading off thickness against more branching connections of structures. In our paper, we use a small value of $h$ (i.e., $10^{-5}$) by default to extract finger cores to preserve more branching connections; also, the extracted thick finger cores are close to the complete volume of fingers, which is beneficial for the extraction of full fingers. We further use the Reeb graph based skeletonization to acquire thin skeletons. 
}

% The scientists can vary this parameter and, from their experience, find a suitable value for $h$. 
% Hence, we use Method One to estimate the derivatives for the finger core extraction. 
% As we decrease $h$ for Method One, the detected features become thicker as well as for the fingering data.
% From the results of the synthetic data in Fig.~\ref{fig:results-synthetic}, when $h$ is equal to the voxel size $s$, the extracted features are ridge voxels. 

\remark{
We offer the theoretical analysis for the spacing parameter $h$. 
% , and discuss the sensitivity of the results to $h$ hereafter.
When changing $h$, we examine how the estimated terms in the gradient vector and the Hessian matrix change accordingly. 
% Finally, we conclude what specific structures are extracted by using different $h$ values. 
We discuss the situations when $h$ is smaller than $s$ and larger than $0$ in the following. 
}

\subsection{Effect of $h$ for Estimated Gradient Vector} \label{app:h_jacobian}
\remark{
Given the center of a voxel, $\vect{p_0}=(x_{1,0}, x_{2,0}, x_{3,0})$, the estimated gradient vector with an additional parameter $h$ at $\vect{p_0}$ is given by 
\begin{equation} \label{equa:jacobian_matrix_h}
\hat{\nabla}f(\vect{p_0}, h) = (f_{x_1}(\vect{p_0}, h), f_{x_2}(\vect{p_0}, h), f_{x_3}(\vect{p_0}, h))^\intercal
\end{equation}
When changing $h$, we analyze how the three components of $\hat{\nabla}f(\vect{p_0}, h)$ change. Without loss of generality, we examine how the component $f_{x_1}(\vect{p_0}, h)$ changes hereafter, where $f_{x_1}(\vect{p_0}, h)$ is defined by Equation~\ref{equa:first_order_derivative_x}. 
% When $h$ equals $s$, $f_{x_1}(\vect{p_0}, h)=f_{x_1}(\vect{p_0},s)=f_{x_1}(x_{1,0},x_{2,0},x_{3,0},s)$. 
We compare $f_{x_1}(\vect{p_0},s)$ and $f_{x_1}(\vect{p_0}, h)$ where $h \in (0,s]$. Note that, for all $h \in (0,s]$, $f(x_{1,0} \pm h, x_{2,0}, x_{3,0})$ are represented by the tri-linear interpolation between $f(x_{1,0}, x_{2,0}, x_{3,0})$ and $f(x_{1,0} \pm s, x_{2,0}, x_{3,0})$. We represent $f(x_{1,0} \pm h, x_{2,0}, x_{3,0})$ by polynomials of $f(x_{1,0}, x_{2,0}, x_{3,0})$ and $f(x_{1,0} \pm s, x_{2,0}, x_{3,0})$ through the formula of the tri-linear interpolation; we substitute the polynomials into Equation~\ref{equa:first_order_derivative_x} and obtain that, $\forall h \in (0,s]$, 
\begin{equation}
f_{x_1}(\vect{p_0},h)=f_{x_1}(\vect{p_0},s)
\end{equation}
Hence, $\forall h \in (0,s]$, 
\begin{equation} \label{equa:jacobian_matrix_h2}
\hat{\nabla}f(\vect{p_0}, h)=\hat{\nabla}f(\vect{p_0}, s)
\end{equation}
In other words, no matter what value of $h \in (0,s]$, the gradient vector $\hat{\nabla}f(\vect{p_0}, h)$ does not change. 
}

\subsection{Effect of $h$ for Estimated Hessian Matrix}
\remark{
We use $\hat{H}(\vect{p_0}, h)$ to represent the Hessian matrix ${H}(\vect{p_0})$ of Equation~\ref{equa:taylor-polynomial}, where $\hat{H}(\vect{p_0}, h)$ is defined by
\begin{equation} \label{equa:hessian_matrix_h}
  \hat{H}(\vect{p_0}, h) = [f_{x_ix_j}(\vect{p_0}, h)],~i,j=1,2,3
\end{equation}
% \begin{align} \label{equa:hessian_matrix_h}
%   \hat{H}(\vect{p_0}, h) =
%   \begin{bmatrix}
%     f_{x_1x_1}(\vect{p_0}, h) & f_{x_1x_2}(\vect{p_0}, h) & f_{x_1x_3}(\vect{p_0}, h) \\
%     f_{x_2x_1}(\vect{p_0}, h) & f_{x_2x_2}(\vect{p_0}, h) & f_{x_2x_3}(\vect{p_0}, h) \\
%     f_{x_3x_1}(\vect{p_0}, h) & f_{x_3x_2}(\vect{p_0}, h) & f_{x_3x_3}(\vect{p_0}, h)
%   \end{bmatrix}
% \end{align}
We analyze how the terms of $\hat{H}(\vect{p_0}, h)$ change when $h$ varies, which is similar to the mathematical analysis of the gradient vector. Without loss of generality, we examine how the terms $f_{x_1x_1}(\vect{p_0}, h)$ and $f_{x_1x_2}(\vect{p_0}, h)$ change hereafter. The central difference formula for $f_{x_1x_1}(\vect{p_0}, h)$ is given by
\begin{dmath} \label{equa:second_order_derivative_xx}
% r_{xx} \approx 
f_{x_1x_1}(\vect{p_0}, h)=f_{x_1x_1}(x_{1,0},x_{2,0},x_{3,0},h) 
= \frac{1}{h^2}(f(x_{1,0}+h,x_{2,0},x_{3,0})-2f(x_{1,0},x_{2,0},x_{3,0})+f(x_{1,0}-h,x_{2,0},x_{3,0}))
\end{dmath}
We represent $f(x_{1,0} \pm h, x_{2,0},x_{3,0})$ by polynomials of $f(x_{1,0},x_{2,0},x_{3,0})$ and $f(x_{1,0} \pm s, x_{2,0},x_{3,0})$ through the formula of the tri-linear interpolation, and obtain that, $\forall h \in (0,s]$, 
\begin{equation}
f_{x_1x_1}(\vect{p_0},h)=\frac{s}{h}f_{x_1x_1}(\vect{p_0},s)
\end{equation}
The central difference formula for $f_{x_1x_2}(\vect{p_0}, h)$ is given by
\begin{dmath} \label{equa:second_order_derivative_xx}
f_{x_1x_2}(\vect{p_0}, h)=f_{x_1x_2}(x_0,y_0,z_0,h)
= \frac{1}{4h^2}(f(x_{1,0}+h,x_{2,0}+h,x_{3,0})
-f(x_{1,0}+h,x_{2,0}-h,x_{3,0})-f(x_{1,0}-h,x_{2,0}+h,x_{3,0})
+f(x_{1,0}-h,x_{2,0}-h,x_{3,0}))
\end{dmath}
We represent $f(x_{1,0} \pm h, x_{2,0} \pm h, x_{3,0})$ by polynomials of $f(x_{1,0}, x_{2,0}, x_{3,0})$ and $f(x_{1,0} \pm s, x_{2,0} \pm s, x_{3,0})$ through the rules of the tri-linear interpolation, and obtain that, $\forall h \in (0,s]$, 
\begin{equation}
f_{x_1x_2}(\vect{p_0},h)=\frac{s}{h}f_{x_1x_2}(\vect{p_0},s)
\end{equation}
Hence, $\forall h \in (0,s]$, 
\begin{equation} \label{equa:hessian_matrix_h2}
\hat{H}(\vect{p_0},h)=\frac{s}{h}\hat{H}(\vect{p_0}, s)
\end{equation}
In other words, the Hessian matrix $\hat{H}(\vect{p_0},h)$ is equal to $\hat{H}(\vect{p_0}, s)$ scaled by $\frac{s}{h}$. Therefore, the eigenvalues of $\hat{H}(\vect{p_0},h)$ are equal to the eigenvalues of $\hat{H}(\vect{p_0},s)$ scaled by $\frac{s}{h}$ for all $h \in (0,s]$; the eigenvectors of $\hat{H}(\vect{p_0},h)$ remain the same. 
}

% \frac{g(x+h,y+h,z)-
% g(x+h,y-h,z)-g(x-h,y+h,z)+g(x-h,y-h,z)}{4h^2} 

\subsection{Effect of $h$ for Ridge Criterion}
\remark{
We analyze the effect of $h$ for Condition One and Two of the ridge criterion demonstrated in Sect.~\ref{sect:ridge_definition} as follows. The second-order Taylor polynomial with the parameter $h$ is 
\begin{dmath} \label{equa:taylor-polynomial-h}
\hat{g}(\vect{p}, h) = 
f(\vect{p_0}) + \hat{\nabla}f(\vect{p_0}, h)^\intercal \vect{\Delta p} + \frac{1}{2}\vect{\Delta p}^\intercal \hat{H}(\vect{p_0}, h) \cdot \vect{\Delta p}
\end{dmath}
where $\vect{\Delta p} = \vect{p} - \vect{p_0}$. 
The gradient vector of $\hat{g}(\vect{p}, h)$ is computed by
\begin{equation} \label{equa:jacobian_matrix_p-h}
\hat{\nabla}g(\vect{p}, h) = \hat{\nabla}f(\vect{p_0}, h) + \hat{H}(\vect{p_0}, h) \cdot \vect{\Delta p}
\end{equation}
}

\subsubsection{Effect of $h$ for Condition One}
\remark{
For Condition One, we compute the first-order directional derivatives of $\hat{g}(\vect{p}, h)$ by 
\begin{equation} \label{equa:directional_derivative_h}
D_{\vec{v_{i}}}\hat{g}(\vect{p}, h) = \vec{v_i}^\intercal \cdot \hat{\nabla}g(\vect{p}, h), ~i=1,2 
\end{equation}
Through Equation~\ref{equa:jacobian_matrix_p-h}, we have 
\begin{equation}\label{equa:directional_derivative_h_expansion}
D_{\vec{v_{i}}}\hat{g}(\vect{p}, h) = \vec{v_i}^\intercal \cdot (\hat{\nabla}f(\vect{p_0}, h) + \hat{H}(\vect{p_0}, h) \cdot \vect{\Delta p}), ~i=1,2 
\end{equation}
}

\remark{We examine whether exists a feature point $\vect{p_1}(h)=(x_{1,1}(h), x_{2,1}(h), x_{3,1}(h))^\intercal$ within the given voxel, where $\vect{p_1}(h)$ is noted as the feature point found by a certain $h$ value. $\vect{\Delta p_1}(h)$ is the displacement of the feature point $\vect{p_1}(h)$ to the center point $\vect{p_0}$, and is given by $\vect{\Delta p_1}(h)=\vect{p_1}(h)-\vect{p_0}$. According to Condition One, we let $D_{\vec{v_{i}}}\hat{g}(\vect{p_1}, h)=0,~i=1,2$. Then, by transforming Equation~\ref{equa:directional_derivative_h_expansion}, $\vect{\Delta p_1}(h)$ satisfies that
\begin{equation} \label{equa:delta_p_condition}
\vec{v_i}^\intercal \cdot \hat{H}(\vect{p_0}, h) \cdot \vect{\Delta p_1}(h)=-\vec{v_i}^\intercal \cdot \hat{\nabla}f(\vect{p_0}, h), ~i=1,2 
\end{equation}
We substitute Equation~\ref{equa:jacobian_matrix_h2} and Equation~\ref{equa:hessian_matrix_h2} into Equation~\ref{equa:delta_p_condition}; hence, $\vect{\Delta p_1}(h)$ satisfies that
\begin{equation} \label{equa:delta_p1_h_condition}
\vec{v_i}^\intercal \cdot \hat{H}(\vect{p_0}, s) \cdot (\frac{s}{h} \vect{\Delta p_1}(h)) =-\vec{v_i}^\intercal \cdot \hat{\nabla}f(\vect{p_0}, s), ~i=1,2 
\end{equation}
Note that, when letting $h$ be $s$ for Equation~\ref{equa:delta_p_condition}, $\vect{\Delta p_1}(s)$ satisfies the following equation
\begin{equation} \label{equa:delta_p1_s_condition}
\vec{v_i}^\intercal \cdot \hat{H}(\vect{p_0}, s) \cdot \vect{\Delta p_1}(s) =-\vec{v_i}^\intercal \cdot \hat{\nabla}f(\vect{p_0}, s), ~i=1,2 
\end{equation}
Hence, by comparing the above two equations, Equation~\ref{equa:delta_p1_h_condition} and \ref{equa:delta_p1_s_condition}, we have $\vect{\Delta p_1}(s) = \frac{s}{h} \vect{\Delta p_1}(h)$, namely, 
\begin{equation} \label{equa:delta_p1_h}
\vect{\Delta p_1}(h) = \frac{h}{s} \vect{\Delta p_1}(s)
\end{equation}
In other words, when $h$ is smaller than or equal to $s$, the feature displacement $\vect{\Delta p_1}(h)$ is equal to the feature displacement $\vect{\Delta p_1}(s)$ scaled by $\frac{h}{s}$, where $\frac{h}{s} \leq 1$. The feature point, $\vect{p_1}(h)=\vect{p_0}+\vect{\Delta p_1}(h)$, is required to be within or on the boundary of the voxel to declare this voxel contains feature points; note that, the region covered by this voxel is a cube centered at $\vect{p_0}$ and has size $s$. Because $\vect{p_1}(s)=\vect{p_0}+\vect{\Delta p_1}(s)=\vect{p_0} + \frac{s}{h} \vect{\Delta p_1}(h)$ through Equation~\ref{equa:delta_p1_h}, it is equivalent to require the ridge point $\vect{p_1}(s)$ to be within or on the boundary of a cube that is centered at $\vect{p_0}$ and has size $\frac{s}{h} \cdot s = \frac{s^2}{h}$. Hence, when using a smaller $h$, the cube size $\frac{s^2}{h}$ becomes larger, and so, it finds the ridge point that is near the voxel yet is outside the voxel. Moreover, as a result, the $r$ in Sect.~\ref{sect:finger_core_extraction} is equal to $\frac{s}{h}$; hence, the adjustment of $h$ produces equivalent results as adjusting $r$. 
% is more likely to find satisfied ridge points.
} 

\subsubsection{Effect of $h$ for Condition Two}
\remark{
We analyze Condition Two. Note that the eigenvalues of $\hat{H}(\vect{p_0},h)$ are equal to the eigenvalues of $\hat{H}(\vect{p_0},s)$ scaled by $\frac{s}{h}$ through Equation~\ref{equa:hessian_matrix_h2}, and the scaling value $\frac{s}{h}$ is positive. Hence, if the eigenvalues of $\hat{H}(\vect{p_0},s)$ are smaller than zero, the eigenvalues of $\hat{H}(\vect{p_0},h), \forall h\in(0,s]$, must be also smaller than zero, and vice versa. In other words, if certain voxels that satisfy Condition Two when $h$ equates $s$, 
then these voxels also satisfy Condition Two when $h\in(0,s]$, and vice versa. 
}
